# Supplementary material for: Night-Rider: Nocturnal Vision-aided Localization in Streetlight Maps Using Invariant Extended Kalman Filtering
Source: arXiv:2402.00330 source file (2024-03-03)
Supplement: Supplementary file 1 [file backup_supplementary_materials.tex]

\documentclass[letterpaper, 10 pt, conference]{ieeeconf}
\IEEEoverridecommandlockouts
\overrideIEEEmargins
% The preceding line is only needed to identify funding in the first footnote. If that is unneeded, please comment it out.
\usepackage{cite}
\usepackage{amsmath,amssymb,amsfonts}
\usepackage{algorithmic}
\usepackage{graphicx}
\usepackage{textcomp}
\usepackage{xcolor}
\usepackage{bm}
\allowdisplaybreaks[4]
%\def\BibTeX{{\rm B\kern-.05em{\sc i\kern-.025em b}\kern-.08em
%    T\kern-.1667em\lower.7ex\hbox{E}\kern-.125emX}}

% ========== format tuning ========== 
% \abovedisplayshortskip=0pt
% \belowdisplayshortskip=0pt
% \abovedisplayskip=3pt
% \belowdisplayskip=3pt
% \setlength{\abovecaptionskip}{3pt}
% \setlength{\belowcaptionskip}{-15pt}

% \setlength{\parskip}{0pt}
% ========== format tuning ========== 

\title{\LARGE \bf
Supplementary Materials: \\ 
Night-Rider: Nocturnal Vision-aided Localization in Streetlight Maps Using Invariant Extended Kalman Filtering 
}


\author{Tianxiao Gao$^{1}$, Mingle Zhao$^{1}$, Chengzhong Xu$^{1}$, and Hui Kong$^{1}$% <-this % stops a space
%\thanks{*This work was not supported by any organization}% <-this % stops a space
\thanks{$^{1}$Tianxiao Gao, Mingle Zhao, Chengzhong Xu and Hui Kong are with the State Key Laboratory of Internet of Things for Smart City (SKL-IOTSC), Faculty of Science and Technology, University of Macau, Macau, China. ({\tt\small \{ga0.tianxiao, zhao.mingle\}@connect.umac.mo, \{czxu, huikong\}@um.edu.mo})}%
}

\begin{document}

\maketitle
\thispagestyle{empty}
\pagestyle{empty}
\setcounter{equation}{26}

This document provides supplementary materials for the ICRA 2024 submission “Night-Rider: Nocturnal Vision-aided Localization in Streetlight Maps Using Invariant Extended Kalman Filtering”.

\subsection{Derivation of Error Propagation Model}
From the Eq. (8), we need to derive the linearized model of right invariant error $\bm{\eta}_{t}^{r}$ and bias error $\bm{\zeta}_{t}$.

For the states fitting into Lie group, the derivative of right invariant error $\bm{\eta}_{t}^{r}$ associates with the log of invariant error $\bm{\xi}_{t}$ based on $\bm{\eta}_{t}^{r}=\exp(\bm{\xi}_{t}^{\wedge})$.
\begin{equation}
\frac{d}{dt}\bm{\eta}_{t}^{r}\approx\frac{d}{dt}(\mathbf{I}+\bm{\xi}_{t}^{\wedge})=\begin{bmatrix}
\frac{d}{dt}(\mathbf{I}+(\bm{\xi}_{R_{t}})_{\times}) & \frac{d}{dt}\bm{\xi}_{v_{t}} & \bm{\xi}_{p_{t}} \\
0 & 0 & 0\\
0 & 0 & 0
\end{bmatrix}
\end{equation}
With Eq. (3), the derivative of $\bm{\xi}_{t}$ is deduced as below.
\begin{align}
&\frac{d}{dt}(\mathbf{I}+(\bm{\xi}_{R_{t}})_{\times})=\frac{d}{dt}(\bm{\xi}_{R_{t}})_{\times}=\frac{d\hat{\mathbf{R}}_{b_{t}}^{w}}{dt}\mathbf{R}_{b_{t}}^{w^{\top}}+\hat{\mathbf{R}}_{b_{t}}^{w}\frac{d\mathbf{R}_{b_{t}}^{w^{\top}}}{dt}\notag\\
&=\hat{\mathbf{R}}_{b_{t}}^{w}(\Tilde{\bm{\omega}}_{t}-\hat{\mathbf{b}}_{\omega_{t}})_{\times}\mathbf{R}_{b_{t}}^{w^{\top}}-\hat{\mathbf{R}}_{b_{t}}^{w}(\bm{\omega}_{t})_{\times}\mathbf{R}_{b_{t}}^{w^{\top}}\notag\\
&=\hat{\mathbf{R}}_{b_{t}}^{w}(\Tilde{\bm{\omega}}_{t}+\mathbf{b}_{\omega_{t}}+\mathbf{n}_{\omega_{t}}-\hat{\mathbf{b}}_{\omega_{t}}-\bm{\omega}_{t})_{\times}\mathbf{R}_{b_{t}}^{w^{\top}}\notag\\
&=\hat{\mathbf{R}}_{b_{t}}^{w}(\mathbf{n}_{\omega_{t}}-\bm{\zeta}_{\omega_{t}})_{\times}\hat{\mathbf{R}}_{b_{t}}^{w^{\top}}\hat{\mathbf{R}}_{b_{t}}^{w}\mathbf{R}_{b_{t}}^{w^{\top}}\notag\\
&=(\hat{\mathbf{R}}_{b_{t}}^{w}(\mathbf{n}_{\omega_{t}}-\bm{\zeta}_{\omega_{t}}))_{\times}\bm{\eta}_{R_{t}}\notag\\
&\approx(\hat{\mathbf{R}}_{b_{t}}^{w}(\mathbf{n}_{\omega_{t}}-\bm{\zeta}_{\omega_{t}}))_{\times}(\mathbf{I}+\bm{\xi}_{R_{t}}) \approx(\hat{\mathbf{R}}_{b_{t}}^{w}(\mathbf{n}_{\omega_{t}}-\bm{\zeta}_{\omega_{t}}))_{\times} \\
%{^{w}}\hat{\mathbf{v}}_{b_{t}} - \hat{\mathbf{R}}_{b_{t}}^{w}\mathbf{R}_{b_{t}}^{w^{\top}} {^{w}}\mathbf{v}_{b_{t}}
&\frac{d}{dt}\bm{\xi}_{v_{t}}=\frac{d}{dt}{^{w}}\hat{\mathbf{v}}_{b_{t}}-\frac{d}{dt}(\hat{\mathbf{R}}_{b_{t}}^{w}\mathbf{R}_{b_{t}}^{w^{\top}}){^{w}}\mathbf{v}_{b_{t}}-\hat{\mathbf{R}}_{b_{t}}^{w}\mathbf{R}_{b_{t}}^{w^{\top}}\frac{d}{dt}{^{w}}\mathbf{v}_{b_{t}}\notag\\
&\approx\hat{\mathbf{R}}_{b_{t}}^{w}(\Tilde{\bm{a}}_{t}-\hat{\mathbf{b}}_{a_{t}})+\mathbf{g}-(\hat{\mathbf{R}}_{b_{t}}^{w}(\mathbf{n}_{\omega_{t}}-\bm{\zeta}_{\omega_{t}}))_{\times}{^{w}}\mathbf{v}_{b_{t}}\notag\\
&\quad - \hat{\mathbf{R}}_{b_{t}}^{w}\mathbf{R}_{b_{t}}^{w^{\top}}(\mathbf{R}_{b_{t}}^{w}\bm{a}_{t}+\mathbf{g})\notag\\
&=\hat{\mathbf{R}}_{b_{t}}^{w}(\bm{a}_{t}+\mathbf{b}_{a_{t}}+\mathbf{n}_{a_{t}}-\hat{\mathbf{b}}_{a_{t}}-\bm{a}_{t})\notag\\
&\quad -(\hat{\mathbf{R}}_{b_{t}}^{w}(\mathbf{n}_{\omega_{t}}-\bm{\zeta}_{\omega_{t}}))_{\times}{^{w}}\mathbf{v}_{b_{t}}+ (\mathbf{I}-\hat{\mathbf{R}}_{b_{t}}^{w}\mathbf{R}_{b_{t}}^{w^{\top}})\mathbf{g}\notag\\
&\approx \hat{\mathbf{R}}_{b_{t}}^{w}(\mathbf{n}_{a_{t}}-\bm{\zeta}_{a_{t}})-(\hat{\mathbf{R}}_{b_{t}}^{w}(\mathbf{n}_{\omega_{t}}-\bm{\zeta}_{\omega_{t}}))_{\times}{^{w}}\mathbf{v}_{b_{t}}-(\bm{\xi}_{R_{t}})_{\times}\mathbf{g}\notag \\
&=(\mathbf{g})_{\times}\bm{\xi}_{R_{t}}+({^{w}}\mathbf{v}_{b_{t}})_{\times}\hat{\mathbf{R}}_{b_{t}}^{w}(\mathbf{n}_{\omega_{t}}-\bm{\zeta}_{\omega_{t}})+\hat{\mathbf{R}}_{b_{t}}^{w}(\mathbf{n}_{a_{t}}-\bm{\zeta}_{a_{t}})\\
%123
&\frac{d}{dt}\bm{\xi}_{p_{t}}=\frac{d}{dt}\hat{\mathbf{p}}_{b_{t}}^{w} -\frac{d}{dt}(\hat{\mathbf{R}}_{b_{t}}^{w}\mathbf{R}_{b_{t}}^{w^{\top}} )\mathbf{p}_{b_{t}}^{w}-\hat{\mathbf{R}}_{b_{t}}^{w}\mathbf{R}_{b_{t}}^{w^{\top}} \frac{d}{dt}\mathbf{p}_{b_{t}}^{w}\notag\\
&\approx{^{w}}\hat{\mathbf{v}}_{b_{t}}-(\hat{\mathbf{R}}_{b_{t}}^{w}(\mathbf{n}_{\omega_{t}}-\bm{\zeta}_{\omega_{t}}))_{\times}\mathbf{p}_{b_{t}}^{w}-\hat{\mathbf{R}}_{b_{t}}^{w}\mathbf{R}_{b_{t}}^{w^{\top}}{^{w}}\mathbf{v}_{b_{t}}\notag\\
&=({^{w}}\hat{\mathbf{v}}_{b_{t}}-\hat{\mathbf{R}}_{b_{t}}^{w}\mathbf{R}_{b_{t}}^{w^{\top}}{^{w}}\mathbf{v}_{b_{t}})-(\hat{\mathbf{R}}_{b_{t}}^{w}(\mathbf{n}_{\omega_{t}}-\bm{\zeta}_{\omega_{t}}))_{\times}\mathbf{p}_{b_{t}}^{w}\notag\\
&=\bm{\xi}_{v_{t}}+(\mathbf{p}_{b_{t}}^{w})_{\times}\hat{\mathbf{R}}_{b_{t}}^{w}(\mathbf{n}_{\omega_{t}}-\bm{\zeta}_{\omega_{t}})
\end{align}
On the other hand, the differential of bias errors is calculated as
\begin{equation}
\frac{d}{dt}\bm{\zeta}_{t}=\begin{bmatrix}
\frac{d}{dt}\hat{\mathbf{b}}_{\omega_{t}} - \frac{d}{dt}\mathbf{b}_{\omega_{t}}\\
\frac{d}{dt}\hat{\mathbf{b}}_{a_{t}} - \frac{d}{dt}\mathbf{b}_{a_{t}}
\end{bmatrix}
=\begin{bmatrix}
\mathbf{n}_{b\omega_{t}}\\
\mathbf{n}_{ba_{t}}
\end{bmatrix}
\end{equation}
Therefore, the linearized model can be written as in Eq. (9).

\subsection{Derivation of $\mathbf{\Sigma}_{t_{proj,ij}}$ and $\sigma^{2}_{t_{ang,ij}}$}
The covariance matrix of reprojection error in Eq. (18) for the streetlight observation $B_{i}$ and cluster $L_{j}$ is derived as below:
\begin{align}
&\mathbf{\Sigma}_{t_{proj,ij}}=\mathbf{\Sigma}_{\Tilde{\mathbf{p}}_{t_{i}}}+\frac{\partial\Tilde{\mathbf{c}}^{m}_{t_{j}}}{\partial\begin{bmatrix}
	\hat{\mathbf{R}}^{w}_{b_{t}} & \hat{\mathbf{p}}^{w}_{b_{t}}
\end{bmatrix}}\hat{\mathbf{P}}_{t}^{-}\left(\frac{\partial\Tilde{\mathbf{c}}^{m}_{t_{j}}}{\partial\begin{bmatrix}
	\hat{\mathbf{R}}^{w}_{b_{t}} & \hat{\mathbf{p}}^{w}_{b_{t}}
	\end{bmatrix}}\right)^{\top}\\
%dc/dR
&\frac{\partial\Tilde{\mathbf{c}}^{m}_{t_{j}}}{\partial \hat{\mathbf{R}}^{w}_{b_{t}}}=\frac{\partial \frac{1}{\Tilde{Z}_{j}^{c}}\mathbf{K}(\mathbf{R}^{c}_{b}\hat{\mathbf{R}}^{w^{\top}}_{b_{t}}(\Tilde{\mathbf{C}}^{w}_{j} - \hat{\mathbf{p}}^{w}_{b_{t}})+\mathbf{t}_{b}^{c})}{\partial \hat{\mathbf{R}^{w}}_{b_{t}}}\notag\\
&\quad\quad\ =\frac{\partial \frac{1}{\Tilde{Z}_{j}^{c}}\mathbf{K}\Tilde{\mathbf{C}}^{c}_{j}}{\partial \hat{\mathbf{R}}^{w}_{b_{t}}}
=\frac{\partial \frac{1}{\Tilde{Z}_{j}^{c}}\mathbf{K}\Tilde{\mathbf{C}}^{c}_{j}}{\partial \Tilde{\mathbf{C}}^{c}_{j}}\frac{\partial \Tilde{\mathbf{C}}^{c}_{j}}{\partial \hat{\mathbf{R}}^{w}_{b_{t}}}\notag\\
&\quad\quad\ =\frac{\partial \frac{1}{\Tilde{Z}_{j}^{c}}\mathbf{K}\Tilde{\mathbf{C}}^{c}_{j}}{\partial \Tilde{\mathbf{C}}^{c}_{j}}\frac{\partial \mathbf{R}^{c}_{b}\hat{\mathbf{R}}^{w^{\top}}_{b_{t}}(\Tilde{\mathbf{C}}^{w}_{j} - \hat{\mathbf{p}}^{w}_{b_{t}})+\mathbf{t}_{b}^{c}}{\partial \hat{\mathbf{R}}^{w}_{b_{t}}}\\
&\quad\quad\ =\begin{bmatrix}
\frac{f_{x}}{\Tilde{Z}^{c}_{j}} & 0 & -\frac{\Tilde{X}^{c}_{j}f_{x}}{\Tilde{Z}^{c^{2}}_{j}}\\
0 & \frac{f_{y}}{\Tilde{Z}^{c}_{j}} & -\frac{\Tilde{Y}^{c}_{j}f_{y}}{\Tilde{Z}^{c^{2}}_{j}}
\end{bmatrix}\mathbf{R}^{c}_{b}(\hat{\mathbf{R}}^{w^{\top}}_{b_{t}}(\Tilde{\mathbf{C}}^{w}_{j}-\hat{\mathbf{p}}^{w}_{b_{t}}))_{\times}\notag\\
%%dc/dt
&\frac{\partial\Tilde{\mathbf{c}}^{m}_{t_{j}}}{\partial \hat{\mathbf{p}}^{w}_{b_{t}}}=\frac{\partial \frac{1}{\Tilde{Z}_{j}^{c}}\mathbf{K}(\mathbf{R}^{c}_{b}\hat{\mathbf{R}}^{w^{\top}}_{b_{t}}(\Tilde{\mathbf{C}}^{w}_{j} - \hat{\mathbf{p}}^{w}_{b_{t}})+\mathbf{t}_{b}^{c})}{\partial \hat{\mathbf{p}}^{w}_{b_{t}}}\notag\\
&\quad\quad\ =\frac{\partial \frac{1}{\Tilde{Z}_{j}^{c}}\mathbf{K}\Tilde{\mathbf{C}}^{c}_{j}}{\partial \hat{\mathbf{p}}^{w}_{b_{t}}}=\frac{\partial \frac{1}{\Tilde{Z}_{j}^{c}}\mathbf{K}\Tilde{\mathbf{C}}^{c}_{j}}{\partial \Tilde{\mathbf{C}}^{c}_{j}}\frac{\partial \Tilde{\mathbf{C}}^{c}_{j}}{\partial \hat{\mathbf{p}}^{w}_{b_{t}}}\notag\\
&\quad\quad\ =\frac{\partial \frac{1}{\Tilde{Z}_{j}^{c}}\mathbf{K}\Tilde{\mathbf{C}}^{c}_{j}}{\partial \Tilde{\mathbf{C}}^{c}_{j}}\frac{\partial \mathbf{R}^{c}_{b}\hat{\mathbf{R}}^{w^{\top}}_{b_{t}}(\Tilde{\mathbf{C}}^{w}_{j} - \hat{\mathbf{p}}^{w}_{b_{t}})+\mathbf{t}_{b}^{c}}{\partial \hat{\mathbf{p}}^{w}_{b_{t}}}\notag\\
&\quad\quad\ =-\begin{bmatrix}
\frac{f_{x}}{\Tilde{Z}^{c}_{j}} & 0 & -\frac{\Tilde{X}^{c}_{j}f_{x}}{\Tilde{Z}^{c^{2}}_{j}}\\
0 & \frac{f_{y}}{\Tilde{Z}^{c}_{j}} & -\frac{\Tilde{Y}^{c}_{j}f_{y}}{\Tilde{Z}^{c^{2}}_{j}}
\end{bmatrix}\mathbf{R}^{c}_{b}\hat{\mathbf{R}}^{w^{\top}}_{b_{t}}
\end{align}
where $\mathbf{\Sigma}_{\Tilde{\mathbf{p}}_{t_{i}}} = \alpha\mathbf{I}_{2\times2}$ and $\alpha$ is a preset parameter. 

Similar to $\mathbf{\Sigma}_{t_{proj,ij}}$, the variance of angle error in Eq. (19) also originates from the covariance of detected streetlight observation and current pose.
\begin{align}
&\sigma^{2}_{t_{ang,ij}}=\frac{\partial\cos\theta_{ij}}{\partial \Tilde{\mathbf{p}}_{t_{i}}}\mathbf{\Sigma}_{\bar{\Tilde{\mathbf{p}}}_{t_{i}}}\left(\frac{\partial\cos\theta_{ij}}{\partial \Tilde{\mathbf{p}}_{t_{i}}}\right)^{\top}\notag\\
&\qquad+\frac{\partial\cos\theta_{ij}}{\partial\begin{bmatrix}
	\mathbf{R}^{w}_{b_{t}} & \mathbf{p}^{w}_{b_{t}}
	\end{bmatrix}}\hat{\mathbf{P}}_{t}^{-}\left(\frac{\partial\cos\theta_{ij}}{\partial\begin{bmatrix}
	\mathbf{R}^{w}_{b_{t}} & \mathbf{p}^{w}_{b_{t}}
	\end{bmatrix}}\right)^{\top}\\
%%dcos/dp
&\frac{\partial\cos\theta_{ij}}{\partial\Tilde{\mathbf{p}}_{t_{i}}}
=\frac{\partial\frac{(\mathbf{K}^{-1}\bar{\Tilde{\mathbf{p}}}_{t_{i}})^{\top}(\mathbf{R}^{c}_{b}\hat{\mathbf{R}}^{w^{\top}}_{b_{t}}(\Tilde{\mathbf{C}}^{w}_{j} - \hat{\mathbf{p}}^{w}_{b_{t}})+\mathbf{t}_{b}^{c})}{\lVert\mathbf{K}^{-1}\bar{\Tilde{\mathbf{p}}}_{t_{i}}\rVert_{2}\cdot\lVert\mathbf{R}^{c}_{b}\hat{\mathbf{R}}^{w^{\top}}_{b_{t}}(\Tilde{\mathbf{C}}^{w}_{j} - \hat{\mathbf{p}}^{w}_{b_{t}})+\mathbf{t}_{b}^{c}\rVert_{2}}}{\partial\Tilde{\mathbf{p}}_{t_{i}}}\notag\\	
&=\frac{\Tilde{\mathbf{C}}_{j}^{c^{\top}}}{\lVert\Tilde{\mathbf{C}}_{j}^{c}\rVert_{2}}\frac{\partial\frac{\Tilde{\mathbf{P}}_{t_{i}}}{\lVert\Tilde{\mathbf{P}}_{t_{i}}\rVert_{2}}}{\partial\Tilde{\mathbf{P}}_{t_{i}}}\frac{\partial\Tilde{\mathbf{P}}_{t_{i}}}{\partial\Tilde{\mathbf{p}}_{t_{i}}}\notag\\
&=\frac{\Tilde{\mathbf{C}}_{j}^{c^{\top}}}{\lVert\Tilde{\mathbf{C}}_{j}^{c}\rVert_{2}}\left(\frac{\mathbf{I}}{\lVert\Tilde{\mathbf{P}}_{t_{i}}\rVert_{2}}-\frac{\Tilde{\mathbf{P}}_{t_{i}}\Tilde{\mathbf{P}}_{t_{i}}^{\top}}{\lVert\Tilde{\mathbf{P}}_{t_{i}}\rVert_{2}^{3}}\right)\mathbf{K}^{-1}\\
%%dcos/dR
&\frac{\partial\cos\theta_{ij}}{\partial\hat{\mathbf{R}}^{w}_{b_{t}}}
=\frac{\partial\frac{(\mathbf{K}^{-1}\bar{\Tilde{\mathbf{p}}}_{t_{i}})^{\top}(\mathbf{R}^{c}_{b}\hat{\mathbf{R}}^{w^{\top}}_{b_{t}}(\Tilde{\mathbf{C}}^{w}_{j} - \hat{\mathbf{p}}^{w}_{b_{t}})+\mathbf{t}_{b}^{c})}{\lVert\mathbf{K}^{-1}\bar{\Tilde{\mathbf{p}}}_{t_{i}}\rVert_{2}\cdot\lVert\mathbf{R}^{c}_{b}\hat{\mathbf{R}}^{w^{\top}}_{b_{t}}(\Tilde{\mathbf{C}}^{w}_{j} - \hat{\mathbf{p}}^{w}_{b_{t}})+\mathbf{t}_{b}^{c}\rVert_{2}}}{\partial\hat{\mathbf{R}}^{w}_{b_{t}}}\notag\\
&=\frac{\Tilde{\mathbf{P}}_{t_{i}}^{\top}}{\lVert\Tilde{\mathbf{P}}_{t_{i}}\rVert_{2}}\frac{\partial\frac{\Tilde{\mathbf{C}}_{j}^{c}}{\lVert\Tilde{\mathbf{C}}_{j}^{c}\rVert_{2}}}{\partial\Tilde{\mathbf{C}}_{j}^{c}}\frac{\partial\Tilde{\mathbf{C}}_{j}^{c}}{\partial\hat{\mathbf{R}}^{w}_{b_{t}}}\notag\\
&=\frac{\Tilde{\mathbf{P}}_{t_{i}}^{\top}}{\lVert\Tilde{\mathbf{P}}_{t_{i}}\rVert_{2}}\left( \frac{\mathbf{I}}{\lVert\Tilde{\mathbf{C}}_{j}^{c}\rVert_{2}} - \frac{\Tilde{\mathbf{C}}_{j}^{c}\Tilde{\mathbf{C}}_{j}^{c^{\top}}}{\lVert\Tilde{\mathbf{C}}_{j}^{c}\rVert_{2}^{3}} \right) \frac{\partial\Tilde{\mathbf{C}}_{j}^{c}}{\partial\hat{\mathbf{R}}^{w}_{b_{t}}}\notag\\
&=\frac{\Tilde{\mathbf{P}}_{t_{i}}^{\top}}{\lVert\Tilde{\mathbf{P}}_{t_{i}}\rVert_{2}}\left( \frac{\mathbf{I}}{\lVert\Tilde{\mathbf{C}}_{j}^{c}\rVert_{2}} - \frac{\Tilde{\mathbf{C}}_{j}^{c}\Tilde{\mathbf{C}}_{j}^{c^{\top}}}{\lVert\Tilde{\mathbf{C}}_{j}^{c}\rVert_{2}^{3}} \right)\mathbf{R}^{c}_{b}(\hat{\mathbf{R}}^{w^{\top}}_{b_{t}}(\Tilde{\mathbf{C}}^{w}_{j}-\hat{\mathbf{p}}^{w}_{b_{t}}))_{\times}\\
%%dcos/dt
&\frac{\partial\cos\theta_{ij}}{\partial\hat{\mathbf{p}}^{w}_{b_{t}}}=\frac{\partial\frac{(\mathbf{K}^{-1}\bar{\Tilde{\mathbf{p}}}_{t_{i}})^{\top}(\mathbf{R}^{c}_{b}\hat{\mathbf{R}}^{w^{\top}}_{b_{t}}(\Tilde{\mathbf{C}}^{w}_{j} - \hat{\mathbf{p}}^{w}_{b_{t}})+\mathbf{t}_{b}^{c})}{\lVert\mathbf{K}^{-1}\bar{\Tilde{\mathbf{p}}}_{t_{i}}\rVert_{2}\cdot\lVert\mathbf{R}^{c}_{b}\hat{\mathbf{R}}^{w^{\top}}_{b_{t}}(\Tilde{\mathbf{C}}^{w}_{j} - \hat{\mathbf{p}}^{w}_{b_{t}})+\mathbf{t}_{b}^{c}\rVert_{2}}}{\partial\hat{\mathbf{p}}^{w}_{b_{t}}}\notag\\
&=\frac{\Tilde{\mathbf{P}}_{t_{i}}^{\top}}{\lVert\Tilde{\mathbf{P}}_{t_{i}}\rVert_{2}}\frac{\partial\frac{\Tilde{\mathbf{C}}_{j}^{c}}{\lVert\Tilde{\mathbf{C}}_{j}^{c}\rVert_{2}}}{\partial\Tilde{\mathbf{C}}_{j}^{c}}\frac{\partial\Tilde{\mathbf{C}}_{j}^{c}}{\partial\hat{\mathbf{p}}^{w}_{b_{t}}}\notag\\
&=\frac{\Tilde{\mathbf{P}}_{t_{i}}^{\top}}{\lVert\Tilde{\mathbf{P}}_{t_{i}}\rVert_{2}}\left( \frac{\mathbf{I}}{\lVert\Tilde{\mathbf{C}}_{j}^{c}\rVert_{2}} - \frac{\Tilde{\mathbf{C}}_{j}^{c}\Tilde{\mathbf{C}}_{j}^{c^{\top}}}{\lVert\Tilde{\mathbf{C}}_{j}^{c}\rVert_{2}^{3}} \right) \frac{\partial\Tilde{\mathbf{C}}_{j}^{c}}{\partial\hat{\mathbf{p}}^{w}_{b_{t}}}\notag\\
&=-\frac{\Tilde{\mathbf{P}}_{t_{i}}^{\top}}{\lVert\Tilde{\mathbf{P}}_{t_{i}}\rVert_{2}}\left( \frac{\mathbf{I}}{\lVert\Tilde{\mathbf{C}}_{j}^{c}\rVert_{2}} - \frac{\Tilde{\mathbf{C}}_{j}^{c}\Tilde{\mathbf{C}}_{j}^{c^{\top}}}{\lVert\Tilde{\mathbf{C}}_{j}^{c}\rVert_{2}^{3}} \right) \mathbf{R}^{c}_{b}\hat{\mathbf{R}}^{w^{\top}}_{b_{t}}
\end{align}
where $\bar{(\cdot)}$ denotes the homogeneous coordinates. $\mathbf{\Sigma}_{\bar{\Tilde{\mathbf{p}}}_{t_{i}}} = diag_block
(\mathbf{I}_{2\times 2}, 0)$.

\subsection{Derivation of the Jacobian Matrix of the Camera-based Observation Model}
For the derivation of the Jacobian matrix $\mathbf{H}_{c_{t_{i}}}$ in Eq. (24), we transform the observation function in Eq. (23) as:
\begin{flalign}\label{observation}
&\mathbf{z}_{c_{t_{i}}}=\mathbf{y}_{t_{i}}-h_{i}(\hat{\mathbf{\Psi}}_{t_{i}})=h_{i}(\mathbf{\Psi}_{t_{i}})-h_{i}(\hat{\mathbf{\Psi}}_{t_{i}})+\mathbf{n}_{c_{t_{i}}}\notag\\
&\approx h_{i}(\hat{\mathbf{\Psi}}_{t_{i}}) + \mathbf{H}_{i}(\mathbf{\hat{\mathbf{\Psi}}_{t_{i}}})(\mathbf{\Psi}_{t_{i}}-\hat{\mathbf{\Psi}}_{t_{i}}) -h_{i}(\hat{\mathbf{\Psi}}_{t_{i}}) +\mathbf{n}_{c_{t_{i}}}\notag\\
&=\mathbf{H}_{i}(\mathbf{\hat{\mathbf{\Psi}}_{t_{i}}})(\mathbf{\Psi}_{t_{i}}-\hat{\mathbf{\Psi}}_{t_{i}})+\mathbf{n}_{c_{t_{i}}}\notag\\
&=\mathbf{H}_{i}(\mathbf{\hat{\mathbf{\Psi}}_{t_{i}}})\left[\mathbf{R}_{b_{t}}^{w^{\top}}(\Tilde{\mathbf{C}}_{t_{j}}^{w}-\mathbf{t}^{w}_{b_{t}})-\hat{\mathbf{R}}_{b_{t}}^{w^{\top}}(\Tilde{\mathbf{C}}_{t_{j}}^{w}-\hat{\mathbf{t}}^{w}_{b_{t}})\right] + \mathbf{n}_{c_{t_{i}}}\notag\\
&=\mathbf{H}_{i}(\mathbf{\hat{\mathbf{\Psi}}_{t_{i}}})\left[\hat{\mathbf{R}}_{b_{t}}^{w^{\top}}(\hat{\mathbf{R}}_{b_{t}}^{w}\mathbf{R}_{b_{t}}^{w^{\top}}-\mathbf{I})\Tilde{\mathbf{C}}_{t_{j}}^{w}\right.\notag\\
&\qquad\qquad\qquad\qquad\qquad\left.+\hat{\mathbf{R}}_{b_{t}}^{w^{\top}}(\hat{\mathbf{t}}^{w}_{b_{t}}-\hat{\mathbf{R}}_{b_{t}}^{w}\mathbf{R}_{b_{t}}^{w^{\top}}\mathbf{t}^{w}_{b_{t}})\right] + \mathbf{n}_{c_{t_{i}}}\notag\\
&\approx -\mathbf{H}_{i}(\mathbf{\hat{\mathbf{\Psi}}_{t_{i}}})\left[\hat{\mathbf{R}}_{b_{t}}^{w^{\top}}(\Tilde{\mathbf{C}}_{t_{j}}^{w})_{\times}\bm{\xi}_{R_{t}}-\hat{\mathbf{R}}_{b_{t}}^{w^{\top}}\bm{\xi}_{p_{t}}\right] + \mathbf{n}_{c_{t_{i}}}&
\end{flalign}
The Jacobian matrix $\mathbf{H}_{i}(\mathbf{\hat{\mathbf{\Psi}}_{t_{i}}})$ is formulated as:
\begin{align}\label{Hi}
&\mathbf{H}_{i}(\hat{\mathbf{\Psi}}_{t_{i}})=\frac{\partial h(\mathbf{\Psi}_{t_{i}})}{\partial \mathbf{\Psi}_{t_{i}}}\Big|_{\mathbf{\Psi}_{t_{i}}=\hat{\mathbf{\Psi}}_{t_{i}}}\notag\\
&=-\frac{1}{\hat{Z}_{t_{j}}^{c^{2}}}(\mathbf{R}_{b}^{c}\hat{\mathbf{\Psi}}_{t_{i}}+\mathbf{t}_{b}^{c})\frac{\partial \hat{Z}_{t_{j}}^{c}}{\partial \mathbf{\Psi}_{t_{i}}}\Big|_{\mathbf{\Psi}_{t_{i}}=\hat{\mathbf{\Psi}}_{t_{i}}}+\frac{1}{\hat{Z}_{t_{j}}^{c}}\mathbf{R}_{b}^{c}\notag \\
&\frac{\partial \hat{Z}_{t_{j}}^{c}}{\partial \mathbf{\Psi}_{t_{i}}}\Big|_{\mathbf{\Psi}_{t_{i}}=\hat{\mathbf{\Psi}}_{t_{i}}}=\frac{\partial \mathbf{R}_{b,3}^{c}\mathbf{\Psi}_{t_{i}}+t_{b,3}^{c}}{\partial \mathbf{\Psi}_{t_{i}}}\Big|_{\mathbf{\Psi}_{t_{i}}=\hat{\mathbf{\Psi}}_{t_{i}}}=\mathbf{R}_{b,3}^{c}
\end{align}
where $\mathbf{R}_{b,3}^{c}$ denotes the third row of $\mathbf{R}_{b}^{c}$ and $t_{b,3}^{c}$ is the third element of $\mathbf{t}_{b}^{c}$. By substituting Eq. (\ref{Hi}) into Eq. (\ref{observation}), the Jacobian matrix $\mathbf{H}_{c_{t_{i}}}$ of the camera-based observation model can be derived. 

\newpage
\begin{align*} 
&\frac{d}{dt} \! \begin{bmatrix} \bm{\xi}_{R_{t}} \\ \bm{\xi}_{v_{t}} \\ \bm{\xi}_{p_{t}} \\ \bm{\zeta}_{\omega_{t}} \\ \bm{\zeta}_{a_{t}} \end{bmatrix} \! = \! \begin{bmatrix} \mathbf{0} & \mathbf{0} & \mathbf{0} & -\hat{\mathbf{R}}_{b_{t}}^{w} & \mathbf{0} \\ (\mathbf{g}^{w})_{\times} & \mathbf{0} & \mathbf{0} & -({^{w}}\hat{\mathbf{v}}_{b_{t}})_{\times} \hat{\mathbf{R}}_{b_{t}}^{w} & -\hat{\mathbf{R}}_{b_{t}}^{w} \\ \mathbf{0} & \mathbf{I} & \mathbf{0} & -(\hat{\mathbf{p}}_{b_{t}}^{w})_{\times} \hat{\mathbf{R}}_{b_{t}}^{w} & \mathbf{0} \\ \mathbf{0} & \mathbf{0} & \mathbf{0} & \mathbf{0} & \mathbf{0} \\ \mathbf{0} & \mathbf{0} & \mathbf{0} & \mathbf{0} & \mathbf{0} \end{bmatrix} 
\begin{bmatrix} \bm{\xi}_{R_{t}} \\ \bm{\xi}_{v_{t}} \\ \bm{\xi}_{p_{t}} \\ \bm{\zeta}_{\omega_{t}} \\ \bm{\zeta}_{a_{t}} \end{bmatrix}+ 
&\! \begin{bmatrix} \hat{\mathbf{R}}_{b_{t}}^{w} & \mathbf{0} & \mathbf{0} & \mathbf{0} & \mathbf{0} \\ ({^{w}}\hat{\mathbf{v}}_{b_{t}})_{\times} \hat{\mathbf{R}}_{b_{t}}^{w} & \hat{\mathbf{R}}_{b_{t}}^{w} & \mathbf{0} & \mathbf{0} & \mathbf{0} \\ (\hat{\mathbf{p}}_{b_{t}}^{w})_{\times} \hat{\mathbf{R}}_{b_{t}}^{w} & \mathbf{0} & \hat{\mathbf{R}}_{b_{t}}^{w} & \mathbf{0} & \mathbf{0} \\ \mathbf{0} & \mathbf{0} & \mathbf{0} & \mathbf{I} & \mathbf{0} \\ \mathbf{0} & \mathbf{0} & \mathbf{0} & \mathbf{0} & \mathbf{I} \end{bmatrix}\! \begin{bmatrix} \mathbf{n}_{\omega_{t}} \\ \mathbf{n}_{a_{t}} \\ \mathbf{0}_{3 \times 1} \\ \mathbf{n}_{b \omega_{t}} \\ \mathbf{n}_{b a_{t}} \end{bmatrix}
% &\triangleq \mathbf{A}_{t} \bm{\xi}_{t} + \mathbf{Ad}_{\hat{\mathbf{X}}_{t}, \hat{\mathbf{b}}_{t}} \mathbf{n}_{t}
\!\triangleq\! \mathbf{A}_{t}\! \begin{bmatrix} \bm{\xi}_{t} \\ \bm{\zeta}_{t} \end{bmatrix}\! +\! \mathbf{Ad}_{\hat{\mathbf{X}}_{t}, \hat{\mathbf{b}}_{t}} \mathbf{n}_{t}
\end{align*}
\begin{equation}
    \mathbf{b}_{t} = \begin{bmatrix} \mathbf{b}_{\omega_{t}} \\
                                      \mathbf{b}_{a_{t}} \end{bmatrix}
\end{equation}

\begin{align}
    \mathbf{z}_{o_{t}} = \begin{bmatrix} \mathbf{0} & \mathbf{I} & \mathbf{0} & \mathbf{0} & \mathbf{0} \end{bmatrix} \begin{bmatrix} \bm{\xi}_{t} \\ \bm{\zeta}_{t} \end{bmatrix} + \hat{\mathbf{R}}_{b_{t}}^{w} \mathbf{n}_{o_{t}} \triangleq -\mathbf{H}_{o_{t}} \begin{bmatrix} \bm{\xi}_{t} \\ \bm{\zeta}_{t} \end{bmatrix} + \hat{\mathbf{R}}_{b_{t}}^{w} \mathbf{n}_{o_{t}}
\end{align}

\begin{align}
    \mathbf{z}_{c_{t_{i}}} = -\mathbf{H}_{i}(\hat{\mathbf{\Psi}}_{t_{i}}) \hat{\mathbf{R}}_{b_{t}}^{w^{\top}} \begin{bmatrix} (\Tilde{\mathbf{C}}_{t_{j}}^{w})_{\times} & \mathbf{0} & -\mathbf{I} & \mathbf{0} & \mathbf{0} \end{bmatrix} \begin{bmatrix} \bm{\xi}_{t} \\ \bm{\zeta}_{t} \end{bmatrix} + \mathbf{n}_{c} \triangleq - \mathbf{H}_{c_{t_{i}}} \begin{bmatrix} \bm{\xi}_{t} \\ \bm{\zeta}_{t} \end{bmatrix} + \mathbf{n}_{c} 
\end{align}

\begin{align}
    &s_{re}=\frac{1}{n_{re}}\sum_{i = 1}^{n_{re}} \Delta p^{b_{re} +}_{i} + \gamma_{1}\Delta t_{b_{re}}^{b_{re} +} + \gamma_{2}\Delta\theta_{b_{re}}^{b_{re} +} + \gamma_{3}\sum_{i=1}^{n_{re}}\!neg(i)\notag\\
    &\Delta p^{b_{re} +}_{i} = \lVert\pi_{c}(\mathbf{R}_{b}^{c} \hat{\mathbf{R}}_{b_{re}}^{{w +}^{\top}}(\Tilde{\mathbf{C}}_{re_{j}}^{w} - \hat{\mathbf{p}}^{w +}_{b_{re}}) + \mathbf{t}_{b}^{c}) - \Tilde{\mathbf{p}}_{re_{i}}\rVert_{2} \notag \\ 
    &\Delta t_{b_{re}}^{b_{re} +} = \lVert\hat{\mathbf{p}}_{b_{re},1,2}^{w -} - \hat{\mathbf{p}}_{b_{re},1,2}^{w +}\rVert_{2} \notag \\ 
    &\Delta \theta_{b_{re}}^{b_{re} +} = yaw(\hat{\mathbf{R}}_{b_{re}}^{{w -}^{\top}}\hat{\mathbf{R}}_{b_{re}}^{w +}) \notag
\end{align}

% \subsection{Proof of Observability}

% \subsection{Implementation Details}

% {
% \bibliographystyle{IEEEtran}
% \bibliography{references}
% }

\end{document}
